# Supplementary material for: S2MDF: A Plug-And-Play Layer for Intersection-Free Multi-Object Signed Distance Fields
Source: arXiv:2605.29761 source file (2026-11-07)
Supplement: Supplementary file 2 [file supp_partsdf_chair.tex]

\begin{table}[ht]
\centering
\resizebox{\textwidth}{!}{%
  \begin{tabular}{c|cccccc}
     & MCD $\downarrow$ & NC $\uparrow$ & F1 (0.001) $\uparrow$ & F1 (0.005) $\uparrow$ & IoU $\uparrow$ & IV $\downarrow$ \\
    \hline
    Vanilla (MC) & 2.644 $\pm$ 6.492 & 96.237 $\pm$ 2.251 & 97.264 $\pm$ 3.441 & 99.307 $\pm$ 1.957 & 89.789 $\pm$ 8.545 & (1.230 $\pm$ 3.704) $\times 10^{-3}$ \\
    \hline
    Min - PP (MC) & 1.393 $\pm$ 2.496 & 96.062 $\pm$ 2.357 & 98.223 $\pm$ 2.066 & 99.721 $\pm$ 0.832 & 92.694 $\pm$ 5.656 & (1.479 $\pm$ 2.620) $\times 10^{-7}$ \\
    Shift - PP (MC) & 1.353 $\pm$ 2.411 & 96.181 $\pm$ 2.312 & 98.282 $\pm$ 2.007 & 99.729 $\pm$ 0.805 & 92.646 $\pm$ 5.705 & (1.917 $\pm$ 5.299) $\times 10^{-8}$ \\
    QP - PP (MC) & 1.358 $\pm$ 2.434 & 96.178 $\pm$ 2.315 & 98.275 $\pm$ 2.015 & 99.728 $\pm$ 0.810 & 92.640 $\pm$ 5.707 & (2.316 $\pm$ 10.350) $\times 10^{-8}$ \\
    \hline
    Min - Train (MC) & 1.510 $\pm$ 2.919 & 96.076 $\pm$ 2.312 & 98.151 $\pm$ 2.124 & 99.681 $\pm$ 0.946 & 92.607 $\pm$ 5.654 & (1.814 $\pm$ 3.617) $\times 10^{-7}$ \\
    Shift - Train (MC) & 1.580 $\pm$ 2.758 & 96.080 $\pm$ 2.279 & 98.060 $\pm$ 2.308 & 99.633 $\pm$ 1.056 & 92.341 $\pm$ 6.179 & (8.743 $\pm$ 17.980) $\times 10^{-8}$ \\
    QP - Train (MC) & 1.687 $\pm$ 4.706 & 96.108 $\pm$ 2.196 & 98.114 $\pm$ 2.229 & 99.653 $\pm$ 1.029 & 92.350 $\pm$ 6.119 & (9.055 $\pm$ 18.070) $\times 10^{-8}$ \\
  \end{tabular}%
}
\caption{PartSDF trained on all chairs in the training set (like in the original paper), tested on different 100 chairs. Mean metrics across shapes and parts (issue in the evaluation, disregard for now).}
\label{tab:supp_partsdf_chair_all}%
\end{table}
