# Supplementary material for: S2MDF: A Plug-And-Play Layer for Intersection-Free Multi-Object Signed Distance Fields
Source: arXiv:2605.29761 source file (2026-11-07)
Supplement: Supplementary file 3 [file supp_objectsdfplus_scenes_all_nobg.tex]

\begin{table}[ht]
\centering
\resizebox{\textwidth}{!}{%
  \begin{tabular}{c|cccc}
     & MCD ($\times 10^{-2}$) $\downarrow$ & NC $\uparrow$ & F1 (0.01) $\uparrow$ & IV $\downarrow$ \\
    \hline
    Vanilla ObjectSDF++ & $9.716 \pm 5.602$ & $77.393 \pm 0.318$ & $66.801 \pm 0.114$ & $(1.447 \pm 0.128) \times 10^{-3}$ \\
    \hline
    \acro{} (QP) - PP & $2.919 \pm 0.866$ & $77.464 \pm 0.202$ & $68.190 \pm 0.198$ & $(1.908 \pm 0.606) \times 10^{-7}$ \\
    \acro{} (Shift-All) - PP & $2.085 \pm 0.236$ & $77.500 \pm 0.188$ & $68.242 \pm 0.182$ & $(1.315 \pm 0.246) \times 10^{-7}$ \\
    \hline
    \acro{} (Shift-All) - Train & $4.730 \pm 1.007$ & $75.861 \pm 0.237$ & $66.710 \pm 0.765$ & $(2.363 \pm 0.206) \times 10^{-7}$ \\
    \acro{} (Shift-All Skip-Conn.) - Train & $3.186 \pm 1.106$ & $77.847 \pm 0.515$ & $68.525 \pm 0.705$ & $(1.550 \pm 1.999) \times 10^{-6}$ \\
  \end{tabular}%
}
\caption{ObjectSDF++~\cite{Wu23b} trained for object-compositional 3D scene reconstruction on 8 Replica~\cite{Straub19} scenes. Mean and standard deviation across 3 runs. Background mesh has been excluded from the evaluation due to the presence of large surfaces outside of the scenes across all methods, which could skew the metrics and make them less informative.}
\label{tab:supp_objectsdfplus_scenes_all_nobg}%
\end{table}
